# Supplementary material for: OnePose: One-Shot Object Pose Estimation without CAD Models
Source: arXiv:2205.12257 source file (2022-05-24)
Supplement: Supplementary file 1 [file supp_ba_align.tex]

\begin{figure}[tb]
    \centering
    \includegraphics[width=\linewidth]{fig/orig_images/supp_ba_align.pdf}
    \caption{
    \textbf{Alignment quality across sequences.} Triangulated point clouds from one sequence are projected to images from another sequence of the same object. 
    The quality of alignment can be measured by the differences between projected 3D points (in blue) and the original 2D keypoints (in red) on the images.
    }
      \vspace{-0.5 cm}
    \label{fig:ba_align}
\end{figure}
