# Supplementary material for: OnePose: One-Shot Object Pose Estimation without CAD Models
Source: arXiv:2205.12257 source file (2022-05-24)
Supplement: Supplementary file 2 [file supp_pvnet.tex]

\begin{figure}[tb]
    \centering
    \includegraphics[width=\linewidth]{fig/orig_images/supp_pvnet_mask.pdf}
    \caption{
    \textbf{Examples of generated masks for PVNet training.} The generated masks are overlayed on the original image in blue.
    }
      \vspace{-0.5 cm}
    \label{fig:mask_example}
\end{figure}
