# Supplementary material for: OnePose: One-Shot Object Pose Estimation without CAD Models
Source: arXiv:2205.12257 source file (2022-05-24)
Supplement: Supplementary file 3 [file supp01_hloc.tex]

\begin{table*}[ht]
    \centering
    \resizebox{\textwidth}{!}{
\begin{tabular}{c||ccc|ccc|ccc|c} 
\hline
\multirow{2}{*}{\#Samples} & \multicolumn{3}{c|}{Large Objects}                  & \multicolumn{3}{c|}{Medium Objects}          & \multicolumn{3}{c|}{Small Objects}          & \multicolumn{1}{l}{\multirow{2}{*}{Time (\textit{ms})}}  \\ 
\cline{2-10}
                             & 1cm-1deg        & 3cm-3deg        & 5cm-5deg        & 1cm-1deg & 3cm-3deg        & 5cm-5deg        & 1cm-1deg & 3cm-3deg        & 5cm-5deg       & \multicolumn{1}{l}{}                                     \\ 
\hline
\multicolumn{11}{c}{HLoc \textit{(SIFT + NN)}}                                                                       \\ 
\hline
2    & 0.214 & 0.418 & 0.449 & 0.292 & 0.489 & 0.519 & 0.177 & 0.357 & 0.398 & 47.79 \\
5     & 0.311 & 0.559 & 0.597 & 0.346 & 0.571 & 0.610 & 0.223 & 0.429 & 0.487 & 116.27
  \\
10    & 0.359 & 0.622 & 0.668 & 0.384 & 0.608 & 0.649 & 0.228 & 0.443 & 0.507 & 218.82   \\
\hline
\multicolumn{11}{c}{HLoc \textit{(SPP + NN)}}                                                                       \\ 
\hline
2     & 0.257 & 0.486 & 0.517 & 0.350 & 0.538 & 0.561 & 0.229 & 0.455 & 0.524 & 54.61\\
5      & 0.333 & 0.618 & 0.661 & 0.425 & 0.654 & 0.693 & 0.304 & 0.576 & 0.651 & 136.98
  \\
10    & 0.388 & 0.682 & 0.730 & 0.464 & 0.707 & 0.747 & 0.325 & 0.609 & 0.705 & 231.89
 \\
\hline
\multicolumn{11}{c}{HLoc \textit{(SPP + SPG)}}                                                                       \\ 
\hline
2                            & 0.308           & 0.553           & 0.584           & 0.438    & 0.618           & 0.628           & 0.294    & 0.542           & 0.619          & 221.43                                                   \\
5                            & 0.426           & 0.789           & 0.835           & 0.541    & 0.779           & 0.815           & 0.390    & 0.711           & 0.822          & 555.56                                                   \\
10                           & 0.479           & 0.846           & 0.879           & 0.580    & 0.839           & 0.869           & 0.422    & 0.754           & 0.876          & 1094.25                                                  \\
\hline
\end{tabular}
}
\caption{\textbf{Experiment on the effects of number of images sampled (i.e., retrieved) for HLoc.} 
We evaluate our visual localization baselines based on HLoc\cite{sarlinCoarseFineRobust2019} with differnt number of images sampled.
}
\label{tab:exp_abl_visloc}
\end{table*}
